# Supplementary material for: DADgraph: A Discourse-aware Dialogue Graph Neural Network for Multiparty Dialogue Machine Reading Comprehension
Source: arXiv:2104.12377 source file (2021-04-26)
Supplement: Supplementary file 1 [file appendix.tex]

\section{Appendices}
\label{sec:appendix}
